# Supplementary material for: A Thermodynamic-Limit Pinning Criterion for Two-Dimensional Structural Superlubricity
Source: arXiv:2607.19732 source file (2026-08-11)
Supplement: Supplementary file 1 [file V1.5-supplement.tex]

\documentclass[reprint,amsmath,amssymb,aps,prb,superscriptaddress,longbibliography]{revtex4-2}
\usepackage{bm}
\usepackage{booktabs}
\usepackage{hyperref}

\newcommand{\dd}{\mathrm{d}}

\newcommand{\Ang}{\text{\AA}}
\newcommand{\Acell}{A_{\rm cell}}

\begin{document}

\title{Supplemental Material for ``A Thermodynamic Pinning Criterion for Two-Dimensional Structural Superlubricity''}
\author{Li Wang}
\affiliation{School of Physics, Nanjing University, Nanjing 210093, China}
\author{Yunjie Ye}
\affiliation{Sichuan ZeroNestor Microelectronics Technology Co., Ltd., Sichuan, China}
\date{\today}
\maketitle

\section{Translation covariance of the smooth continuum}

Let the registry-dependent part of a defect-free continuum functional be
\begin{equation}
E_{\rm int}[\bm u,\bm X]
=\int_A\dd^2r\,
V_{\rm GSFE}[-B\bm r+\bm X+\bm u(\bm r)],
\end{equation}
with a translationally invariant elastic energy and $\langle\bm u\rangle_A=0$. For nonsingular mismatch matrix $B$, choose $\bm a=B^{-1}\Delta\bm X$ and define
\begin{equation}
\bm u_{\bm X+\Delta\bm X}(\bm r)
=\bm u_{\bm X}(\bm r-\bm a).
\end{equation}
Changing variables to $\bm r'=\bm r-\bm a$ leaves the bulk energy density unchanged. The finite-boundary difference is subextensive for boundary sequences that restore translation invariance. Thus a smooth infinite moir\'e continuum has a continuous translated family of equal-energy textures even after nonlinear reconstruction. If $B$ is rank deficient, the argument protects only shifts in $\operatorname{Im}B$; a complementary commensurate channel requires a separate depinning test. Atomic sampling, an edge, a defect, or an external field also breaks the covariance used in the proof.

\section{Published graphene/hBN input}

The DMC adhesion potential of Szyniszewski \emph{et al.} is \cite{Szyniszewski2025}
\begin{equation}
V_A(\bm\ell)=v_{s0}
+v_{s1}\sum_{j=1}^{3}\cos(\bm G_j\cdot\bm\ell)
+v_{as1}\sum_{j=1}^{3}\sin(\bm G_j\cdot\bm\ell),
\end{equation}
where
\begin{equation}
\begin{aligned}
v_{s0}&=-57(3)~{\rm meV/cell},\\
v_{s1}&=2.2(3)~{\rm meV/cell},\qquad
v_{as1}=-3.5(4)~{\rm meV/cell}.
\end{aligned}
\end{equation}
For the convention
\begin{equation}
V_{\rm GSFE}=\sum_{j=1}^{3}
\left[E_Ge^{i\bm G_j\cdot\bm\ell}+{\rm c.c.}\right],
\end{equation}
coefficient matching gives
\begin{equation}
E_G=(v_{s1}-iv_{as1})/2=(1.10+i1.75)~{\rm meV/cell}.
\end{equation}
The magnitude $2.067~{\rm meV/cell}$ is smaller than the $15~{\rm meV/cell}$ energy lowering associated with replacing a translationally averaged interface by the optimal uniform stacking. These quantities have different definitions and cannot be interchanged.

The lattice constants are $a_{\rm G}=2.462~{\rm \Ang}$ and $a_{\rm hBN}=2.504~{\rm \Ang}$. The graphene elastic constants are $C_{11}=352.6$, $C_{12}=59.6$, and $C_{66}=146.5~{\rm N/m}$ \cite{Liu2016Elastic}; the hBN values are $293.2$, $66.1$, and $113.55~{\rm N/m}$ \cite{Peng2012}. For two free layers the longitudinal and transverse relative moduli are harmonic combinations of the layer moduli. For rigid hBN only the graphene compliance enters.

\section{Leven-2016 interlayer-potential spectrum}

To test the first-star truncation independently, we implement the C--B and C--N interlayer potential of Leven \emph{et al.} directly from their Table I \cite{Leven2016}. For atoms $i$ and $j$ on opposing layers,
\begin{align}
V_{ij}={}&{\rm Tap}(r_{ij})
\Bigg\{e^{-\alpha_{ij}(r_{ij}/\beta_{ij}-1)}\nonumber\\
&\quad\times\left[\epsilon_{ij}+C_{ij}
\left(e^{-(\rho_{ij}/\gamma_{ij})^2}
+e^{-(\rho_{ji}/\gamma_{ij})^2}\right)\right]\nonumber\\
&-\frac{C_{6,ij}}{r_{ij}^6}
\left[1+e^{-d(r_{ij}/(s_R\,r_{ij}^{\rm eff})-1)}\right]^{-1}
\Bigg\},
\label{eq:leven_ilp}
\end{align}
where ${\rm Tap}(r)$ is the seventh-order cutoff polynomial that vanishes at $R_{\rm cut}=16~{\rm \Ang}$. For flat layers, $\rho_{ij}=\rho_{ji}$ is the lateral pair separation. The exact parameters used are listed in Table~\ref{tab:leven_parameters}.
\begin{table*}[t]
\caption{Leven-2016 graphene/hBN ILP parameters used to generate the local sliding surface. Lengths are in \Ang, $C_6$ in ${\rm kcal\,\Ang^6/mol}$, and $\epsilon,C$ in ${\rm kcal/mol}$. Both pairs use $d=15.0$ and $s_R=0.784$.}
\label{tab:leven_parameters}
\begin{ruledtabular}
\begin{tabular}{lccccccc}
Pair & $r^{\rm eff}$ & $C_6$ & $\alpha$ & $\beta$ & $\gamma$ & $\epsilon$ & $C$ \\
\hline
C--B & 3.691 & 657.408 & 10.0 & 3.02 & 1.2 & 0.37 & 0.18 \\
C--N & 3.481 & 366.955 & 10.0 & 3.40 & 1.2 & 0.21 & 0.36 \\
\end{tabular}
\end{ruledtabular}
\end{table*}

Following the published sliding calculation, we evaluate a flat commensurate local bilayer at $z=3.3~{\rm \Ang}$ on a $48\times48$ shift grid. Its peak-to-trough corrugation is $30.4198~{\rm meV}$ per graphene cell. We transform the grid according to
\begin{equation}
V(s,t)=V_0+\sum_{(h,k)\in\mathcal H}
\left[A_{hk}\cos 2\pi(hs+kt)+B_{hk}\sin 2\pi(hs+kt)\right].
\end{equation}
Retaining the 15 reciprocal pairs with amplitude at least $10^{-5}$ of the largest coefficient gives an rms reconstruction error of $3.26\times10^{-5}~{\rm meV/cell}$. The largest complex coefficient, $|(A_{hk}-iB_{hk})/2|=3.08570~{\rm meV/cell}$, is $49.3\%$ larger than the DMC first-star value. Repeating the construction on a $32\times32$ grid changes the corrugation by $0.205\%$ and the largest coefficient by less than the stored numerical precision. The generated grid, retained spectrum, source metadata, and selection threshold are stored in \texttt{ghbn\_leven2016\_gsfe.json}.

\section{Discrete model and Fourier normalization}

The real-space sites are $\bm R_{mn}=m\bm a_1+n\bm a_2$, with $0\le m,n<N$. For mismatch $p/N$, the substrate phase at an unrelaxed graphene site is, modulo $2\pi$,
\begin{equation}
(\varphi_1,\varphi_2,\varphi_3)
=\frac{2\pi p}{N}(-m,-n,m+n).
\end{equation}
The total energy for either adhesion spectrum is
\begin{align}
E={}&\frac{A}{2}\sum_{\bm q\ne0}
u_i^*(\bm q)D_{ij}(\bm q)u_j(\bm q)\nonumber\\
&+g\sum_{mn}\sum_{\alpha\in\mathcal H}
\left[A_\alpha\cos\Phi_{\alpha mn}+B_\alpha\sin\Phi_{\alpha mn}\right],
\end{align}
where
\begin{equation}
\Phi_{\alpha mn}=\varphi_{\alpha mn}
+\bm G_\alpha\cdot(\bm X+\bm u_{mn}).
\end{equation}
For the DMC model, $\mathcal H$ contains the three first-star vectors and $(A_\alpha,B_\alpha)=(v_{s1},v_{as1})$. For the Leven model, each $\bm G_\alpha=h\bm b_1+k\bm b_2$ and the corresponding $(A_{hk},B_{hk})$ is read from the generated spectrum.
The discrete Fourier transform is normalized by
\begin{equation}
\bm u_{\bm q}=N^{-2}\sum_{mn}\bm u_{mn}e^{-i\bm q\cdot\bm R_{mn}}.
\end{equation}
With this convention the code evaluates the elastic energy as
\begin{equation}
E_{\rm el}=\frac{\Acell}{2N^2}
\sum_{\bm q}\bm F_{\bm q}^{\dagger}D(\bm q)\bm F_{\bm q},
\end{equation}
where $\bm F_{\bm q}$ is the unnormalized forward transform. The corresponding real-space gradient is $\Acell$ times the inverse transform of $D\bm F$. This normalization was independently checked by finite differences.

For isotropic hexagonal elasticity,
\begin{equation}
D_{ij}(\bm q)=C_Tq^2\delta_{ij}+(C_L-C_T)q_iq_j.
\end{equation}
The code uses a spectral inverse-square-root of $\Acell D+\kappa I$ as an optimization preconditioner. The positive $\kappa$ is set by the retained adhesion curvature and does not enter the physical energy.

\section{Primitive sliding period}

For coprime $p,N$, shifting $\bm X$ by $\bm h/N$, where $\bm h=h_1\bm a_1+h_2\bm a_2$, is equivalent to a lattice translation by the modular inverse of $p$ multiplied by $(h_1,h_2)$. Therefore the primitive relaxed-energy period along this path is $|\bm h|/N$. This is shorter than the substrate primitive vector. Sampling a full vector only at shifts commensurate with $N$ evaluates symmetry-equivalent points and can falsely return a zero corrugation.

The sampled direction indices were
\begin{equation}
(1,0),\ (3,1),\ (2,1),\ (3,2),\ (1,1),
\end{equation}
covering the irreducible $0^\circ$--$30^\circ$ sector. Each primitive period was sampled at 24 equally spaced shifts.

The physical-coupling calculation uses three increasing approximants, $p/N=1/60$, $2/119$, and $3/179$. The corresponding supercells contain $3600$, $14161$, and $32041$ displacement sites. The same approximants are used in the full shift-torus audit below.

\section{Stationary-state search}

At each imposed shift, L-BFGS first locates the local basin in preconditioned variables. The result is polished by damped Newton--CG. For perturbation $\delta\bm u$, the adhesion part of the Hessian action is
\begin{equation}
\begin{aligned}
(H_{\rm int}\delta\bm u)_{mn}
=g\sum_j&[-v_{s1}\cos\Phi_{jmn}-v_{as1}\sin\Phi_{jmn}]\\
&\times\bm G_j(\bm G_j\cdot\delta\bm u_{mn}).
\end{aligned}
\end{equation}
The elastic Hessian action is evaluated spectrally. The uniform displacement mode is removed from the field, gradient, search direction, and Hessian action.

For the DMC multi-start test, random mean-zero initial fields had component standard deviations $0.1$, $0.3$, $0.6$, and $1.0~{\rm \Ang}$. All endpoints were compared in both energy and root-mean-square field distance. No symmetry-inequivalent endpoint was found at physical coupling. Repeating the same 25-start protocol for each boundary condition with the Leven spectrum gives 50 converged endpoints, an energy spread no larger than $1.49\times10^{-15}~{\rm meV/cell}$, and a maximum rms separation from the lowest endpoint below $5.0\times10^{-16}~{\rm \Ang}$. No second Leven minimum is found.

\section{Tilted-enthalpy continuation}

For a continuously followed local minimum with branch energy $E_m(X)$, the enthalpy density along a sampled path is
\begin{equation}
h_{m,\tau}(X)=E_m(X)/A-\tau X.
\end{equation}
Stationary points obey
\begin{equation}
\frac{1}{A}\frac{\partial E_m}{\partial X}=\tau.
\end{equation}
The effective curvature after eliminating internal coordinates is
\begin{equation}
\kappa_{\rm eff}
=E_{XX}-E_{Xu}H_{uu}^{-1}E_{uX}.
\end{equation}
We locate every stationary root over one primitive period, retain roots with $\kappa_{\rm eff}>0$, and follow the root connected to the zero-stress minimum. The terminal saddle-node has $\kappa_{\rm eff}=0$. A threshold is accepted only when it exceeds the independently defined force--energy consistency scale.

No physical-$g=1$ branch terminates above that scale. At artificial strong coupling, the $N=60$ branches terminate at $1.434\times10^{-6}~{\rm MPa}$ for $g=40$ and $2.1268\times10^{-3}~{\rm MPa}$ for $g=80$. Their normalized curvatures decrease continuously to zero, as shown in Fig.~2(d) of the main text. The corresponding larger approximants have no resolved saddle-node.

\section{Complete physical-coupling summary}

\begin{table*}[t]
\caption{Maxima over the five sampled directions at $g=1$. A stress is unresolved whenever it is below $\epsilon_\tau$.}
\begingroup
\footnotesize
\setlength{\tabcolsep}{4pt}
\begin{ruledtabular}
\begin{tabular}{lcccccc}
boundary & $p/N$ & $\Lambda$ & max. $|\bm u|$ (\AA) & max. strain & max. $\tau_{\rm energy}$ (MPa) & $\epsilon_\tau^{\max}$ (MPa) \\
\hline
free/free & $1/60$ & 0.14187 & 0.1696 & 0.784\% & $2.42\times10^{-11}$ & $1.65\times10^{-9}$ \\
free/free & $2/119$ & 0.13952 & 0.1669 & 0.776\% & $2.49\times10^{-11}$ & $2.60\times10^{-9}$ \\
free/free & $3/179$ & 0.14030 & 0.1678 & 0.779\% & $2.98\times10^{-11}$ & $2.22\times10^{-9}$ \\
rigid hBN & $1/60$ & 0.06441 & 0.0779 & 0.338\% & $8.74\times10^{-12}$ & $1.68\times10^{-8}$ \\
rigid hBN & $2/119$ & 0.06334 & 0.0766 & 0.334\% & $1.52\times10^{-11}$ & $7.59\times10^{-10}$ \\
rigid hBN & $3/179$ & 0.06370 & 0.0770 & 0.336\% & $1.85\times10^{-11}$ & $2.81\times10^{-9}$ \\
\end{tabular}
\end{ruledtabular}
\endgroup
\end{table*}

The Fourier-derived energy corrugations are at the numerical precision floor. Direct forces are more sensitive to incomplete cancellation and therefore set the conservative upper bounds. None of these direct-force residuals is interpreted as a positive friction signal.

\section{Two-dimensional shift-torus result}

The primitive collective-shift torus is sampled as
\begin{equation}
\bm X_{ij}=\frac{i}{12}\frac{\bm a_1}{N}
+\frac{j}{12}\frac{\bm a_2}{N},
\qquad 0\le i,j<12.
\end{equation}
For each of the six size--boundary combinations, all 144 internal minimizations pass the projected-gradient criterion. A two-dimensional Fourier transform of $E_{\min}(\bm X)/A$ gives the Cartesian restoring-stress field and hence $\Phi_R$. The direct stress is retained as an independent consistency estimator, not as a positive signal.

\begin{table*}[t]
\caption{Physical-coupling DMC first-star shift-torus audit. All stress columns are in MPa.}
\begingroup
\footnotesize
\setlength{\tabcolsep}{4pt}
\begin{ruledtabular}
\begin{tabular}{lccccc}
boundary & $p/N$ & $\Phi_R^{\rm energy}$ & $\tau_{\rm eq,max}^{\rm energy}$ & $\epsilon_{\rm torus}$ & status \\
\hline
free/free & $1/60$ & $4.96\times10^{-12}$ & $1.26\times10^{-11}$ & $3.41\times10^{-9}$ & unresolved \\
free/free & $2/119$ & $7.98\times10^{-12}$ & $2.04\times10^{-11}$ & $1.83\times10^{-10}$ & unresolved \\
free/free & $3/179$ & $1.12\times10^{-11}$ & $2.50\times10^{-11}$ & $4.61\times10^{-10}$ & unresolved \\
rigid hBN & $1/60$ & $3.72\times10^{-12}$ & $9.14\times10^{-12}$ & $3.35\times10^{-10}$ & unresolved \\
rigid hBN & $2/119$ & $4.78\times10^{-12}$ & $1.23\times10^{-11}$ & $2.87\times10^{-10}$ & unresolved \\
rigid hBN & $3/179$ & $7.73\times10^{-12}$ & $1.60\times10^{-11}$ & $9.24\times10^{-10}$ & unresolved \\
\end{tabular}
\end{ruledtabular}
\endgroup
\end{table*}

The corresponding Leven-spectrum results are listed in Table~\ref{tab:leven_torus}.
\begin{table*}[t]
\caption{Physical-coupling Leven-spectrum shift-torus audit. All stress columns are in MPa.}
\label{tab:leven_torus}
\begingroup
\footnotesize
\setlength{\tabcolsep}{4pt}
\begin{ruledtabular}
\begin{tabular}{lccccc}
boundary & $p/N$ & $\Phi_R^{\rm energy}$ & $\tau_{\rm eq,max}^{\rm energy}$ & $\epsilon_{\rm torus}$ & status \\
\hline
free/free & $1/60$ & $1.61\times10^{-11}$ & $4.03\times10^{-11}$ & $2.04\times10^{-9}$ & unresolved \\
free/free & $2/119$ & $1.68\times10^{-11}$ & $3.87\times10^{-11}$ & $4.91\times10^{-10}$ & unresolved \\
free/free & $3/179$ & $4.57\times10^{-11}$ & $1.24\times10^{-10}$ & $4.32\times10^{-10}$ & unresolved \\
rigid hBN & $1/60$ & $1.07\times10^{-11}$ & $2.66\times10^{-11}$ & $1.00\times10^{-10}$ & unresolved \\
rigid hBN & $2/119$ & $1.43\times10^{-11}$ & $2.87\times10^{-11}$ & $2.73\times10^{-10}$ & unresolved \\
rigid hBN & $3/179$ & $1.90\times10^{-11}$ & $5.16\times10^{-11}$ & $1.27\times10^{-8}$ & unresolved \\
\end{tabular}
\end{ruledtabular}
\endgroup
\end{table*}

The spectral values in every row of both audits lie below the force--energy consistency scale. Therefore neither adhesion landscape resolves a nonzero $\Phi_R$ or a maximum equilibrium restoring stress on the sampled torus.

\section{Strong-coupling finite-size data}

\begin{table*}[t]
\caption{Free/free strong-coupling audit along $\bm a_1$.}
\begingroup
\footnotesize
\setlength{\tabcolsep}{4pt}
\begin{ruledtabular}
\begin{tabular}{ccccccc}
$g$ & $p/N$ & $\Lambda$ & max. strain & corrugation (meV/cell) & $\tau_{\rm energy}$ (MPa) & status \\
\hline
20 & $1/60$ & 2.84 & 9.49\% & $7.28\times10^{-14}$ & $1.81\times10^{-9}$ & unresolved \\
20 & $2/119$ & 2.79 & 9.48\% & $5.46\times10^{-14}$ & $1.83\times10^{-9}$ & unresolved \\
40 & $1/60$ & 5.67 & 14.17\% & $6.25\times10^{-10}$ & $1.44\times10^{-6}$ & resolved \\
40 & $2/119$ & 5.58 & 14.15\% & $7.28\times10^{-14}$ & $5.21\times10^{-9}$ & unresolved \\
80 & $1/60$ & 11.35 & 20.70\% & $9.23\times10^{-7}$ & $2.13\times10^{-3}$ & resolved \\
80 & $2/119$ & 11.16 & 20.69\% & $1.94\times10^{-10}$ & $7.43\times10^{-6}$ & unresolved \\
80 & $3/179$ & 11.22 & 20.69\% & $2.93\times10^{-11}$ & $1.81\times10^{-6}$ & unresolved \\
\end{tabular}
\end{ruledtabular}
\endgroup
\end{table*}

The local-strain growth invalidates a quantitative harmonic-elastic interpretation before a size-independent barrier is observed. Consequently these data cannot be fitted to a critical-scaling collapse and do not define $g_c$.

\section{Corner--edge--bulk finite-size extrapolation}

For a fixed flake shape and aspect ratio, we fit the static depinning force to
\begin{equation}
F_{\rm dep}(A)=a_{\rm c}+b_{\rm e}A^{1/2}+c_{\rm s}A+o(A^{1/2}).
\end{equation}
The corresponding stress is
\begin{equation}
\tau_{\rm dep}(A)=a_{\rm c}A^{-1}+b_{\rm e}A^{-1/2}+c_{\rm s}+o(A^{-1/2}),
\end{equation}
so the thermodynamic order parameter is the static area coefficient $c_{\rm s}=\tau_{\rm dep}^{\rm bulk}$, not the finite force. Gao \emph{et al.} report $F_s=b_{\rm e}A^{1/2}$ upper and lower envelopes for polygonal graphene/hBN flakes \cite{Gao2025Edge}. Their published coefficients, with $F_s$ in nN and $A$ in ${\rm nm^2}$, are listed in Table~\ref{tab:gao_edge_coefficients}.
\begin{table}[t]
\caption{Static edge-envelope coefficients transcribed from Fig.~4 of Ref.~\cite{Gao2025Edge}.}
\label{tab:gao_edge_coefficients}
\begin{ruledtabular}
\begin{tabular}{lcc}
Shape & lower $b_{\rm e}$ & upper $b_{\rm e}$ \\
\hline
Rectangle & 0.65 & 1.34 \\
Square & 0.75 & 1.76 \\
Hexagon & 0.60 & 1.922 \\
Triangle & 1.70 & 2.68 \\
\end{tabular}
\end{ruledtabular}
\end{table}
After division by area, every reported edge envelope decays as $A^{-1/2}$. A nonzero bulk floor $c_{\rm s}$ overtakes it at $A_\times=(b_{\rm e}/c_{\rm s})^2$ in consistent units. The script \texttt{ghbn\_edge\_bulk\_extrapolation.py} records this conversion and the stress flow without refitting plotted data. Gao \emph{et al.} use $a_k+b_kA^{1/2}+c_kA$ for kinetic friction; its $c_k$ is a dissipative surface term and is not interchangeable with the static coefficient $c_{\rm s}$.

\section{Dimensional consistency}

The displacement $\bm u$ has units of length, while $\bm G$, $\bm q$, and the sliding-spectrum vector $\bm K$ have units of inverse length. Both the GSFE coefficient $V_G$ and the two-dimensional elastic moduli have units of energy per area. Since $D(\bm q)=Cq^2$, the elastic kernel has units of energy per length to the fourth power, and
\begin{equation}
|V_G|G_i[D^{-1}(\bm q)]_{ij}G_j
\end{equation}
is dimensionless. The spectral diagnostic $\Phi_R=[\sum_{\bm K\ne0}K^2|V^{\rm ren}_{\bm K}|^2]^{1/2}$ has units of energy per volume, equivalent to force per area and hence to shear stress.

\section{Reproducibility and scope}

The accompanying calculation repository contains the source DOI and Fourier convention, every optimizer report, direct and energy-derived stresses, period-closure errors, displacement and strain diagnostics, and machine-readable DMC--Leven and Gao-scaling summaries. The calculation is zero-temperature and defect-free and uses in-plane harmonic elasticity with either the DMC first star or the 15-harmonic fixed-height Leven spectrum. No claim is made about nonlinear elasticity, dynamically relaxed interlayer height, finite-flake chemistry, polycrystals, pressure, or thermal creep.

The numerical result is a null detection of pinning in the two specified in-plane models, not an experimental zero-friction prediction. All 30 size--direction--boundary paths, six $12\times12$ shift tori, and 50 multi-start endpoints have been evaluated for each adhesion model. Tilted-enthalpy continuation has been completed for all resolved DMC branches found by the constrained searches. A mathematically exhaustive phase assignment would still require a dense angular limit, exclusion of remote branches outside the present search basin, and a fully atomistic out-of-plane calculation.

\bibliographystyle{apsrev4-2}
\bibliography{superlubricity-v15}

\end{document}
