# Supplementary material for: A Thermodynamic-Limit Pinning Criterion for Two-Dimensional Structural Superlubricity
Source: arXiv:2607.19732 source file (2026-08-11)
Supplement: Supplementary file 2 [file V1.6-arxiv-supplement.tex]

\documentclass[reprint,amsmath,amssymb,aps,prb,superscriptaddress,longbibliography]{revtex4-2}
\usepackage{bm}
\usepackage{graphicx}
\usepackage{booktabs}
\usepackage{hyperref}

\newcommand{\dd}{\mathrm{d}}
\newcommand{\ii}{\mathrm{i}}
\newcommand{\Ang}{\text{\AA}}
\newcommand{\Acell}{A_{\rm cell}}

\begin{document}

\title{Supplemental Material for ``A Thermodynamic Pinning Criterion for Two-Dimensional Structural Superlubricity''}
\author{Li Wang}
\affiliation{School of Physics, Nanjing University, Nanjing 210093, China}
\author{Yunjie Ye}
\affiliation{Sichuan ZeroNestor Microelectronics Technology Co., Ltd., Sichuan, China}
\date{\today}
\maketitle

\section{Translation covariance of the smooth continuum}

Let the registry-dependent part of a defect-free continuum functional over a two-dimensional domain of area $A$ be
\begin{equation}
E_{\rm int}[\bm u,\bm X]
=\int_A\dd^2r\,
V_{\rm GSFE}[B\bm r+\bm X+\bm u(\bm r)],
\end{equation}
where $B$ maps real-space position to local stacking displacement, $\bm X$ is the collective interlayer shift, and $\bm u(\bm r)$ is the internal relative-displacement field. The elastic energy is translationally invariant, and the zero mode is fixed by $\langle\bm u\rangle_A=A^{-1}\int_A\dd^2r\,\bm u(\bm r)=0$. For nonsingular $B$, choose $\bm a=B^{-1}\Delta\bm X$ and define
\begin{equation}
\bm u_{\bm X+\Delta\bm X}(\bm r)
=\bm u_{\bm X}(\bm r+\bm a).
\end{equation}
Changing variables to $\bm r'=\bm r+\bm a$ leaves both bulk terms and the bulk energy density unchanged. The finite-boundary energy and force differences are subextensive for boundary sequences that restore translation invariance. Thus a smooth infinite moir\'e continuum has a continuous translated family of equal-energy textures even after nonlinear reconstruction. If $B$ is rank deficient, the argument protects only shifts in $\operatorname{Im}B$; a complementary commensurate channel requires a separate depinning test. Atomic sampling, an edge, a defect, or an external field also breaks the covariance used in the proof.

\section{Published graphene/hBN input}

The diffusion quantum Monte Carlo (DMC) adhesion potential of Szyniszewski \emph{et al.} is \cite{Szyniszewski2025}
\begin{equation}
V_A(\bm\ell)=v_{s0}
+v_{s1}\sum_{j=1}^{3}\cos(\bm G_j\cdot\bm\ell)
+v_{as1}\sum_{j=1}^{3}\sin(\bm G_j\cdot\bm\ell),
\end{equation}
where $\bm\ell$ is the local interlayer shift, $\bm G_j$ are the three inequivalent vectors in the first reciprocal-lattice star of the local commensurate stacking cell, and $V_A$ is the adhesion energy per graphene primitive basis. The fitted coefficients are
\begin{equation}
\begin{aligned}
v_{s0}&=-57(3)~{\rm meV/cell},\\
v_{s1}&=2.2(3)~{\rm meV/cell},\qquad
v_{as1}=-3.5(4)~{\rm meV/cell}.
\end{aligned}
\end{equation}
Parentheses denote one-standard-deviation statistical uncertainties in the last quoted digits.
For the convention, with c.c. denoting the complex-conjugate term,
\begin{equation}
V_{\rm GSFE}=\sum_{j=1}^{3}
\left[E_Ge^{\ii\bm G_j\cdot\bm\ell}+{\rm c.c.}\right],
\end{equation}
coefficient matching gives
\begin{equation}
E_G=(v_{s1}-\ii v_{as1})/2=(1.10+\ii1.75)~{\rm meV/cell}.
\end{equation}
The corresponding GSFE coefficient per area is $V_G=E_G/\Acell$, where $\Acell=\sqrt{3}a_{\rm G}^2/2$ is the graphene primitive-cell area. The magnitude $|E_G|=2.067~{\rm meV/cell}$ is smaller than the $15~{\rm meV/cell}$ energy lowering associated with replacing a translationally averaged interface by the optimal uniform stacking. These quantities have different definitions and cannot be interchanged.

The lattice constants are $a_{\rm G}=2.462~{\rm \Ang}$ and $a_{\rm hBN}=2.504~{\rm \Ang}$. The graphene elastic constants are $C_{11}=352.6$, $C_{12}=59.6$, and $C_{66}=146.5~{\rm N/m}$ \cite{Liu2016Elastic}; the hBN values are $293.2$, $66.1$, and $113.55~{\rm N/m}$ \cite{Peng2012}. For two free layers the longitudinal and transverse relative moduli are harmonic combinations of the layer moduli. For rigid hBN only the graphene compliance enters.

\section{Leven-2016 interlayer-potential spectrum}

To test the first-star truncation independently, we implement the C--B and C--N interlayer potential of Leven \emph{et al.} directly from their Table I \cite{Leven2016}. For atoms $i$ and $j$ on opposing layers,
\begin{align}
V_{ij}={}&{\rm Tap}(r_{ij})
\Bigg\{e^{-\alpha_{ij}(r_{ij}/\beta_{ij}-1)}\nonumber\\
&\quad\times\left[\epsilon_{ij}+C_{ij}
\left(e^{-(\rho_{ij}/\gamma_{ij})^2}
+e^{-(\rho_{ji}/\gamma_{ij})^2}\right)\right]\nonumber\\
&-\frac{C_{6,ij}}{r_{ij}^6}
\left[1+e^{-d(r_{ij}/(s_R\,r_{ij}^{\rm eff})-1)}\right]^{-1}
\Bigg\},
\label{eq:leven_ilp}
\end{align}
Here $r_{ij}=|\bm r_j-\bm r_i|$ is the interatomic distance and
$\rho_{ij}^2=r_{ij}^2-[\bm n_i\cdot(\bm r_j-\bm r_i)]^2$ is the squared distance transverse to the local normal $\bm n_i$; $\rho_{ji}$ is defined analogously using $\bm n_j$. Thus $\rho_{ij}=\rho_{ji}$ is the lateral pair separation for flat, parallel layers. The dimensionless switching function $\mathrm{Tap}(r)$ is the seventh-order cutoff polynomial of Ref.~\cite{Leven2016} and vanishes at $R_{\rm cut}=16~{\rm \Ang}$. The parameters $\alpha_{ij}$, $d$, and $s_R$ are dimensionless; $\beta_{ij}$, $\gamma_{ij}$, and $r_{ij}^{\rm eff}$ are lengths; $\epsilon_{ij}$ and $C_{ij}$ are energies; and $C_{6,ij}$ has units of energy times length to the sixth power. The exact parameters used are listed in Table~\ref{tab:leven_parameters}.
Writing $x=r/R_{\rm cut}$, the implemented cutoff is
\begin{equation}
\mathrm{Tap}(r)=
\begin{cases}
1-35x^4+84x^5-70x^6+20x^7,&x<1,\\
0,&x\ge1.
\end{cases}
\label{eq:leven_taper}
\end{equation}
\begin{table*}[t]
\caption{Leven-2016 graphene/hBN ILP parameters used to generate the local sliding surface. Lengths are in \Ang, $C_6$ in ${\rm kcal\,\Ang^6/mol}$, and $\epsilon,C$ in ${\rm kcal/mol}$. Both pairs use $d=15.0$ and $s_R=0.784$.}
\label{tab:leven_parameters}
\begin{ruledtabular}
\begin{tabular}{lccccccc}
Pair & $r^{\rm eff}$ & $C_6$ & $\alpha$ & $\beta$ & $\gamma$ & $\epsilon$ & $C$ \\
\hline
C--B & 3.691 & 657.408 & 10.0 & 3.02 & 1.2 & 0.37 & 0.18 \\
C--N & 3.481 & 366.955 & 10.0 & 3.40 & 1.2 & 0.21 & 0.36 \\
\end{tabular}
\end{ruledtabular}
\end{table*}

Following the published sliding calculation, we evaluate a flat commensurate local bilayer at interlayer separation $z=3.3~{\rm \Ang}$ and local lattice constant $a_0=2.504~{\rm \Ang}$ on a $48\times48$ shift grid. The local cell contains the two-atom graphene basis above one B--N primitive basis, and its energy is the sum of Eq.~\eqref{eq:leven_ilp} over all opposing-layer pairs inside the cutoff. Its area is $A_0=\sqrt{3}a_0^2/2=5.42999~{\rm \Ang^2}$, and its peak-to-trough corrugation is $30.4198~{\rm meV}$ per local cell, or $5.60218~{\rm meV/\Ang^2}$. Writing the local shift as $\bm\ell=s\bm a_1^{(0)}+t\bm a_2^{(0)}$, with $0\le s,t<1$ and commensurate primitive vectors $\bm a_1^{(0)},\bm a_2^{(0)}$, we transform the grid according to
\begin{equation}
V(s,t)=V_0+\sum_{(h,k)\in\mathcal H}
\left[\mathcal C_{hk}\cos 2\pi(hs+kt)+\mathcal S_{hk}\sin 2\pi(hs+kt)\right].
\end{equation}
Here $V_0$ is the shift average, $(h,k)$ are integer reciprocal indices, $\mathcal H$ is the retained set containing one member of each $\pm(h,k)$ pair, and $\mathcal C_{hk},\mathcal S_{hk}$ are real energies per local cell. Retaining the 15 reciprocal pairs whose complex amplitudes $\tfrac12(\mathcal C_{hk}-\ii\mathcal S_{hk})$ are at least $10^{-5}$ of the largest amplitude gives a root-mean-square (rms) reconstruction error of $3.26\times10^{-5}~{\rm meV/cell}$. The largest complex coefficient, $|\mathcal C_{hk}-\ii\mathcal S_{hk}|/2=3.08570~{\rm meV/cell}$, is $49.3\%$ larger than the DMC first-star value. Repeating the construction on a $32\times32$ grid changes the corrugation by $0.205\%$ and the largest coefficient by less than the stored numerical precision. The generated grid, retained spectrum, source metadata, and selection threshold are stored in \texttt{ghbn\_leven2016\_gsfe.json}.
The reconstructed sliding surface and retained Fourier spectrum are shown in Fig.~\ref{fig:s_model_audit}(a,b).

\section{Discrete model and Fourier normalization}

The $N\times N$ periodic graphene sampling lattice contains sites $\bm R_{mn}=m\bm a_1^{\rm G}+n\bm a_2^{\rm G}$, with $0\le m,n<N$, total area $A=N^2\Acell$, and displacement $\bm u_{mn}=\bm u(\bm R_{mn})$. For the zero-twist approximant $\delta_N=p/N$, the substrate vectors are $\bm a_i^{\rm S}=\bm a_i^{\rm G}/(1-\delta_N)$, and $\bm b_i^{\rm S}$ are their reciprocal vectors. A retained adhesion harmonic $\alpha\in\mathcal H$ has $\bm G_\alpha=h\bm b_1^{\rm S}+k\bm b_2^{\rm S}$ and unrelaxed phase
\begin{equation}
\varphi_{\alpha mn}=\bm G_\alpha\cdot B\bm R_{mn}
\pmod{2\pi}.
\end{equation}
For mismatch $p/N$, the phases of the three DMC first-star vectors are
\begin{equation}
(\varphi_{1mn},\varphi_{2mn},\varphi_{3mn})
=\frac{2\pi p}{N}(-m,-n,m+n)
\pmod{2\pi}.
\end{equation}
The total energy for either retained adhesion spectrum is
\begin{align}
E={}&\frac{A}{2}\sum_{\bm q\ne0}
u_i^*(\bm q)D_{ij}(\bm q)u_j(\bm q)\nonumber\\
&+g\sum_{mn}\sum_{\alpha\in\mathcal H}
\left[\mathcal C_\alpha\cos\Phi_{\alpha mn}
+\mathcal S_\alpha\sin\Phi_{\alpha mn}\right],
\end{align}
where
\begin{equation}
\Phi_{\alpha mn}=\varphi_{\alpha mn}
+\bm G_\alpha\cdot(\bm X+\bm u_{mn}).
\end{equation}
Here $\bm X$ is the imposed collective shift, $g$ is a dimensionless adhesion multiplier whose physical value is $g=1$, and $\mathcal C_\alpha,\mathcal S_\alpha$ are adhesion energies assigned per graphene sampling site. For the DMC model, $\mathcal H$ contains the three first-star vectors and $(\mathcal C_\alpha,\mathcal S_\alpha)=(v_{s1},v_{as1})$. For the Leven model, $(\mathcal C_\alpha,\mathcal S_\alpha)=(\mathcal C_{hk},\mathcal S_{hk})$ is read from the generated spectrum. The Leven per-local-cell energies are retained on transfer to this common graphene sampling lattice; energy densities and $\Lambda$ then use the graphene area $\Acell$, not the local grid area $A_0$.
The discrete Fourier transform is normalized by
\begin{equation}
\bm u_{\bm q}=N^{-2}\sum_{mn}\bm u_{mn}e^{-\ii\bm q\cdot\bm R_{mn}}.
\end{equation}
The wave vectors $\bm q$ run over the reciprocal grid of the periodic $N\times N$ supercell; the $\bm q=0$ mode is removed by $N^{-2}\sum_{mn}\bm u_{mn}=0$. Defining the unnormalized transform $\bm F_{\bm q}=N^2\bm u_{\bm q}$, the code evaluates the elastic energy as
\begin{equation}
E_{\rm el}=\frac{\Acell}{2N^2}
\sum_{\bm q}\bm F_{\bm q}^{\dagger}D(\bm q)\bm F_{\bm q},
\end{equation}
where $\dagger$ denotes Hermitian conjugation. The corresponding real-space gradient is $\Acell$ times the inverse transform of $D\bm F$. This normalization was independently checked by finite differences.

For isotropic hexagonal elasticity,
\begin{equation}
D_{ij}(\bm q)=C_Tq^2\delta_{ij}+(C_L-C_T)q_iq_j.
\end{equation}
Here $C_L$ and $C_T$ are the longitudinal and transverse moduli appropriate to the chosen free/free or rigid-hBN boundary condition, and $\delta_{ij}$ is the Kronecker delta. The code uses the spectral inverse square root of $\Acell D+\kappa I$ as an optimization preconditioner, where $I$ is the $2\times2$ identity in displacement space and the positive numerical regularizer $\kappa$ has units of energy per length squared. It is set from the retained adhesion curvature and does not enter the physical energy.

\section{Primitive sliding period}

Let $p$ and $N$ be coprime, and let $p^{-1}$ denote the multiplicative inverse of $p$ modulo $N$. For an integer substrate vector $\bm h=h_1\bm a_1^{\rm S}+h_2\bm a_2^{\rm S}$, shifting $\bm X$ by $\bm h/N$ is equivalent, modulo the periodic supercell, to translating the graphene sampling lattice by $p^{-1}(h_1,h_2)$. Therefore the primitive relaxed-energy period along the unit direction $\hat{\bm h}=\bm h/|\bm h|$ is $|\bm h|/N$. This period is shorter than a substrate primitive vector. Sampling only shifts commensurate with a full substrate period can revisit symmetry-equivalent points and falsely return zero corrugation.

The sampled direction indices were
\begin{equation}
(1,0),\ (3,1),\ (2,1),\ (3,2),\ (1,1),
\end{equation}
covering the irreducible $0^\circ$--$30^\circ$ sector. Each primitive period was sampled at 24 equally spaced shifts.
The label $(r,s)$ denotes $\bm h=r\bm a_1^{\rm S}+s\bm a_2^{\rm S}$; the five vectors are primitive because their integer components are coprime.

The physical-coupling calculation uses three increasing approximants, $p/N=1/60$, $2/119$, and $3/179$. The corresponding supercells contain $3600$, $14161$, and $32041$ displacement sites. The same approximants are used in the full shift-torus audit below.

\section{Stationary-state search}

At each imposed shift, the limited-memory Broyden--Fletcher--Goldfarb--Shanno (L-BFGS) algorithm first locates a local basin in preconditioned variables. The result is polished by damped Newton--conjugate-gradient (Newton--CG) iteration. For a displacement perturbation $\delta\bm u$, the adhesion part of the Hessian action for either retained spectrum is
\begin{equation}
\begin{aligned}
(H_{\rm int}\delta\bm u)_{mn}
=g\sum_{\alpha\in\mathcal H}
&[-\mathcal C_\alpha\cos\Phi_{\alpha mn}
-\mathcal S_\alpha\sin\Phi_{\alpha mn}]\\
&\times\bm G_\alpha
(\bm G_\alpha\cdot\delta\bm u_{mn}).
\end{aligned}
\end{equation}
Here $H_{\rm int}$ is the adhesion Hessian with respect to all site displacements. The elastic Hessian action is evaluated spectrally. The uniform displacement mode is removed from the field, gradient, search direction, and Hessian action.

For the DMC multi-start test, random mean-zero initial fields had component standard deviations $0.1$, $0.3$, $0.6$, and $1.0~{\rm \Ang}$. All endpoints were compared in both energy and root-mean-square field distance. No symmetry-inequivalent endpoint was found at physical coupling. Repeating the same 25-start protocol for each boundary condition with the Leven spectrum gives 50 converged endpoints, an energy spread no larger than $1.49\times10^{-15}~{\rm meV/cell}$, and a maximum rms separation from the lowest endpoint below $5.0\times10^{-16}~{\rm \Ang}$. No second Leven minimum is found.

\section{Tilted-enthalpy continuation}

Choose a sampled unit direction $\hat{\bm e}$ and write the unwrapped collective coordinate as $\bm X=X\hat{\bm e}$, where the scalar $X$ has units of length. For a continuously followed local minimum with branch energy $E_m(X)$, the tilted enthalpy density under the projected shear stress $\tau$ is
\begin{equation}
h_{m,\tau}(X)=E_m(X)/A-\tau X.
\end{equation}
Stationary points obey
\begin{equation}
\frac{1}{A}\frac{\partial E_m}{\partial X}=\tau.
\end{equation}
The effective curvature after eliminating internal coordinates is
\begin{equation}
\kappa_{\rm eff}
=E_{XX}-E_{Xu}H_{uu}^{-1}E_{uX}.
\end{equation}
Here $E_{XX}=\partial^2E/\partial X^2$, $E_{Xu}$ and $E_{uX}$ are the mixed derivative row and column blocks, and $H_{uu}$ is the Hessian with respect to the mean-zero internal displacement coordinates; all blocks are evaluated at the stationary branch. Thus $\kappa_{\rm eff}=\dd^2E_m/\dd X^2$ has units of energy per length squared. We locate every stationary root over one primitive period, retain roots with $\kappa_{\rm eff}>0$, and follow the root connected to the zero-stress minimum. The terminal saddle-node has $\kappa_{\rm eff}=0$. A threshold is accepted only when it exceeds the force--energy consistency scale $\epsilon_\tau$ defined below.

No physical-$g=1$ branch terminates above that scale. At artificial strong coupling, the $N=60$ branches terminate at $1.434\times10^{-6}~{\rm MPa}$ for $g=40$ and $2.1268\times10^{-3}~{\rm MPa}$ for $g=80$. Their curvatures, normalized by the corresponding zero-stress values $\kappa_0=\kappa_{\rm eff}(\tau=0)$, decrease continuously to zero, as shown in Fig.~2(d) of the main text. The corresponding larger approximants have no resolved saddle-node.

\section{Complete physical-coupling summary}

Along each path, let $\tau_{\rm force}=A^{-1}\hat{\bm e}\cdot\partial E/\partial\bm X$ be the direct generalized stress, and let $\tau_{\rm energy}$ be the derivative of the Fourier representation of $E_{\min}(X)/A$. The physical restoring stress is their negative; the sign is immaterial to the absolute-value diagnostics and consistency residuals below. With $\langle\cdots\rangle_X$ denoting the average over the 24 shifts in one primitive period, the pre-registered pathwise resolution is
\begin{equation}
\epsilon_\tau=
\max\!\left[
5\left\langle
(\tau_{\rm force}-\tau_{\rm energy})^2
\right\rangle_X^{1/2},
10^{-10}~{\rm MPa}
\right].
\label{eq:supp_path_resolution}
\end{equation}
The table reports $\epsilon_\tau^{\max}$, the largest pathwise value over the five sampled directions for a given size and boundary condition. A stress is resolved only when it exceeds its own pathwise $\epsilon_\tau$.
For harmonic $\alpha$, define $\bm q_\alpha=B^T\bm G_\alpha$ and the continuum coefficient $V_\alpha=(\mathcal C_\alpha-\ii\mathcal S_\alpha)/(2\Acell)$. The reconstruction susceptibility reported below is
\begin{equation}
\Lambda=\max_{\alpha\in\mathcal H}
|V_\alpha|G_{\alpha i}
[D^{-1}(\bm q_\alpha)]_{ij}G_{\alpha j}.
\label{eq:supp_lambda}
\end{equation}
The maximum strain is the largest absolute component of $\varepsilon_{ij}=(\partial_i u_j+\partial_j u_i)/2$ over the supercell, and $\max|\bm u|$ is the largest site-displacement magnitude.

\begin{table*}[t]
\caption{DMC first-star maxima over the five sampled directions at $g=1$. A stress is unresolved whenever it is below $\epsilon_\tau$.}
\label{tab:physical_summary}
\begingroup
\footnotesize
\setlength{\tabcolsep}{4pt}
\begin{ruledtabular}
\begin{tabular}{lcccccc}
boundary & $p/N$ & $\Lambda$ & max. $|\bm u|$ (\AA) & max. strain & max. $\tau_{\rm energy}$ (MPa) & $\epsilon_\tau^{\max}$ (MPa) \\
\hline
free/free & $1/60$ & 0.14187 & 0.1696 & 0.784\% & $2.42\times10^{-11}$ & $1.65\times10^{-9}$ \\
free/free & $2/119$ & 0.13952 & 0.1669 & 0.776\% & $2.49\times10^{-11}$ & $2.60\times10^{-9}$ \\
free/free & $3/179$ & 0.14030 & 0.1678 & 0.779\% & $2.98\times10^{-11}$ & $2.22\times10^{-9}$ \\
rigid hBN & $1/60$ & 0.06441 & 0.0779 & 0.338\% & $8.74\times10^{-12}$ & $1.68\times10^{-8}$ \\
rigid hBN & $2/119$ & 0.06334 & 0.0766 & 0.334\% & $1.52\times10^{-11}$ & $7.59\times10^{-10}$ \\
rigid hBN & $3/179$ & 0.06370 & 0.0770 & 0.336\% & $1.85\times10^{-11}$ & $2.81\times10^{-9}$ \\
\end{tabular}
\end{ruledtabular}
\endgroup
\end{table*}

Table~\ref{tab:physical_summary} shows that the Fourier-derived energy corrugations are at the numerical precision floor. Direct forces are more sensitive to incomplete cancellation and therefore set the conservative upper bounds. None of these direct-force residuals is interpreted as a positive friction signal.

Figure~\ref{fig:s_directional_audit} reports the complete direction-resolved comparison in dimensionless form. Dividing the energy-derived stress by the pre-registered resolution avoids comparing raw residuals obtained from different system sizes and optimization conditions. Every matrix element is below unity and hence unresolved.

\section{Two-dimensional shift-torus result}

The primitive collective-shift torus is sampled as
\begin{equation}
\bm X_{ij}=\frac{i}{12}\frac{\bm a_1^{\rm S}}{N}
+\frac{j}{12}\frac{\bm a_2^{\rm S}}{N},
\qquad 0\le i,j<12.
\end{equation}
Here $i$ and $j$ are integer grid indices, and $\bm a_1^{\rm S}/N,\bm a_2^{\rm S}/N$ span the primitive collective-shift cell $\Omega_X$. For each of the six size--boundary combinations, all 144 internal minimizations pass the projected-gradient criterion. We write the Fourier representation of the relaxed energy density as
\begin{equation}
\frac{E_{\min}(\bm X)}{A}
=\overline e+\sum_{\bm K\ne0}
V_{\bm K}^{\rm ren}e^{\ii\bm K\cdot\bm X},
\end{equation}
where $\overline e$ is the shift average and $\bm K$ runs over the reciprocal grid of $\Omega_X$. Spectral differentiation gives
\begin{equation}
\begin{aligned}
\bm\tau_{\rm energy}(\bm X)
&=\bm\nabla_{\bm X}
\left[\frac{E_{\min}(\bm X)}{A}\right],\\
\Phi_R
&=\left[
\sum_{\bm K\ne0}K^2|V_{\bm K}^{\rm ren}|^2
\right]^{1/2}.
\end{aligned}
\end{equation}
We denote the maximum spectral stress magnitude on the grid by $\tau_{\rm eq,max}^{\rm energy}=\max_{\bm X}|\bm\tau_{\rm energy}(\bm X)|$. The direct relaxed generalized stress $\bm\tau_{\rm force}=A^{-1}\partial E/\partial\bm X$ is retained as an independent consistency estimator; the restoring stress has the opposite sign. With $\langle\cdots\rangle_{\Omega_X}$ denoting the average over the 144 shifts, the torus resolution is
\begin{equation}
\begin{aligned}
\epsilon_{\rm torus}=\max\!\Bigl[
&5\bigl\langle
|\bm\tau_{\rm force}-\bm\tau_{\rm energy}|^2
\bigr\rangle_{\Omega_X}^{1/2},\\
&10^{-10}~{\rm MPa}
\Bigr].
\end{aligned}
\label{eq:supp_torus_resolution}
\end{equation}
Neither the direct-stress residual nor any spectral value below $\epsilon_{\rm torus}$ is interpreted as a positive signal.

The DMC first-star torus results are listed in Table~\ref{tab:dmc_torus}.
\begin{table*}[t]
\caption{Physical-coupling DMC first-star shift-torus audit. All stress columns are in MPa.}
\label{tab:dmc_torus}
\begingroup
\footnotesize
\setlength{\tabcolsep}{4pt}
\begin{ruledtabular}
\begin{tabular}{lccccc}
boundary & $p/N$ & $\Phi_R^{\rm energy}$ & $\tau_{\rm eq,max}^{\rm energy}$ & $\epsilon_{\rm torus}$ & status \\
\hline
free/free & $1/60$ & $4.96\times10^{-12}$ & $1.26\times10^{-11}$ & $3.41\times10^{-9}$ & unresolved \\
free/free & $2/119$ & $7.98\times10^{-12}$ & $2.04\times10^{-11}$ & $1.83\times10^{-10}$ & unresolved \\
free/free & $3/179$ & $1.12\times10^{-11}$ & $2.50\times10^{-11}$ & $4.61\times10^{-10}$ & unresolved \\
rigid hBN & $1/60$ & $3.72\times10^{-12}$ & $9.14\times10^{-12}$ & $3.35\times10^{-10}$ & unresolved \\
rigid hBN & $2/119$ & $4.78\times10^{-12}$ & $1.23\times10^{-11}$ & $2.87\times10^{-10}$ & unresolved \\
rigid hBN & $3/179$ & $7.73\times10^{-12}$ & $1.60\times10^{-11}$ & $9.24\times10^{-10}$ & unresolved \\
\end{tabular}
\end{ruledtabular}
\endgroup
\end{table*}

The corresponding Leven-spectrum results are listed in Table~\ref{tab:leven_torus}.
\begin{table*}[t]
\caption{Physical-coupling Leven-spectrum shift-torus audit. All stress columns are in MPa.}
\label{tab:leven_torus}
\begingroup
\footnotesize
\setlength{\tabcolsep}{4pt}
\begin{ruledtabular}
\begin{tabular}{lccccc}
boundary & $p/N$ & $\Phi_R^{\rm energy}$ & $\tau_{\rm eq,max}^{\rm energy}$ & $\epsilon_{\rm torus}$ & status \\
\hline
free/free & $1/60$ & $1.61\times10^{-11}$ & $4.03\times10^{-11}$ & $2.04\times10^{-9}$ & unresolved \\
free/free & $2/119$ & $1.68\times10^{-11}$ & $3.87\times10^{-11}$ & $4.91\times10^{-10}$ & unresolved \\
free/free & $3/179$ & $4.57\times10^{-11}$ & $1.24\times10^{-10}$ & $4.32\times10^{-10}$ & unresolved \\
rigid hBN & $1/60$ & $1.07\times10^{-11}$ & $2.66\times10^{-11}$ & $1.00\times10^{-10}$ & unresolved \\
rigid hBN & $2/119$ & $1.43\times10^{-11}$ & $2.87\times10^{-11}$ & $2.73\times10^{-10}$ & unresolved \\
rigid hBN & $3/179$ & $1.90\times10^{-11}$ & $5.16\times10^{-11}$ & $1.27\times10^{-8}$ & unresolved \\
\end{tabular}
\end{ruledtabular}
\endgroup
\end{table*}

The spectral values in every row of both audits lie below the force--energy consistency scale. Therefore neither adhesion landscape resolves a nonzero $\Phi_R$ or a maximum equilibrium restoring stress on the sampled torus.

\begin{figure*}[t]
\centering
\includegraphics[width=0.98\textwidth]{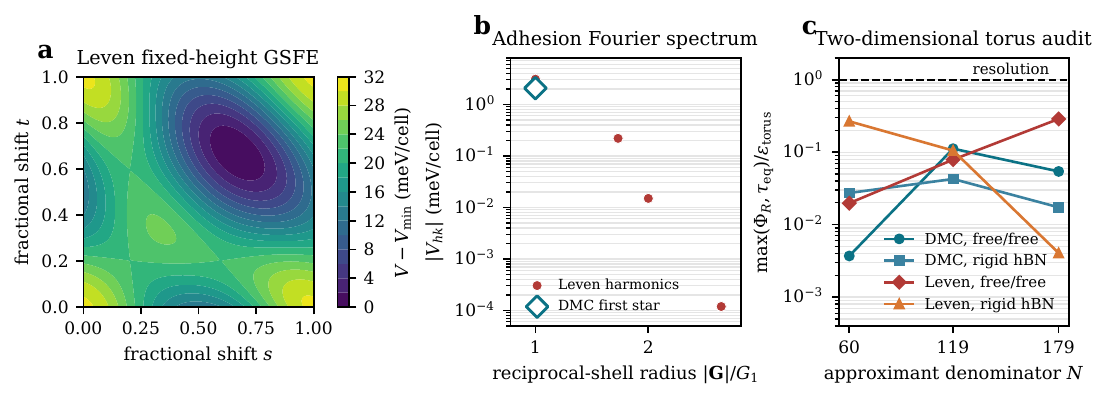}
\caption{
Adhesion-model and two-dimensional equilibrium audit.
(a) Fixed-height Leven-2016 graphene/hBN sliding surface reconstructed from the 15 retained reciprocal pairs; the zero is the minimum energy on the shift cell.
(b) Magnitudes of the retained Leven complex Fourier coefficients compared with the independent DMC first-star coefficient. The higher shells are smaller but are retained in every Leven discrete calculation.
(c) Largest energy-derived equilibrium diagnostic divided by its independently defined force--energy resolution for the two adhesion spectra, both boundary conditions, and all three approximants. A resolved signal would lie above the dashed line; every tested point remains below it.
}
\label{fig:s_model_audit}
\end{figure*}

\begin{figure*}[t]
\centering
\includegraphics[width=0.88\textwidth]{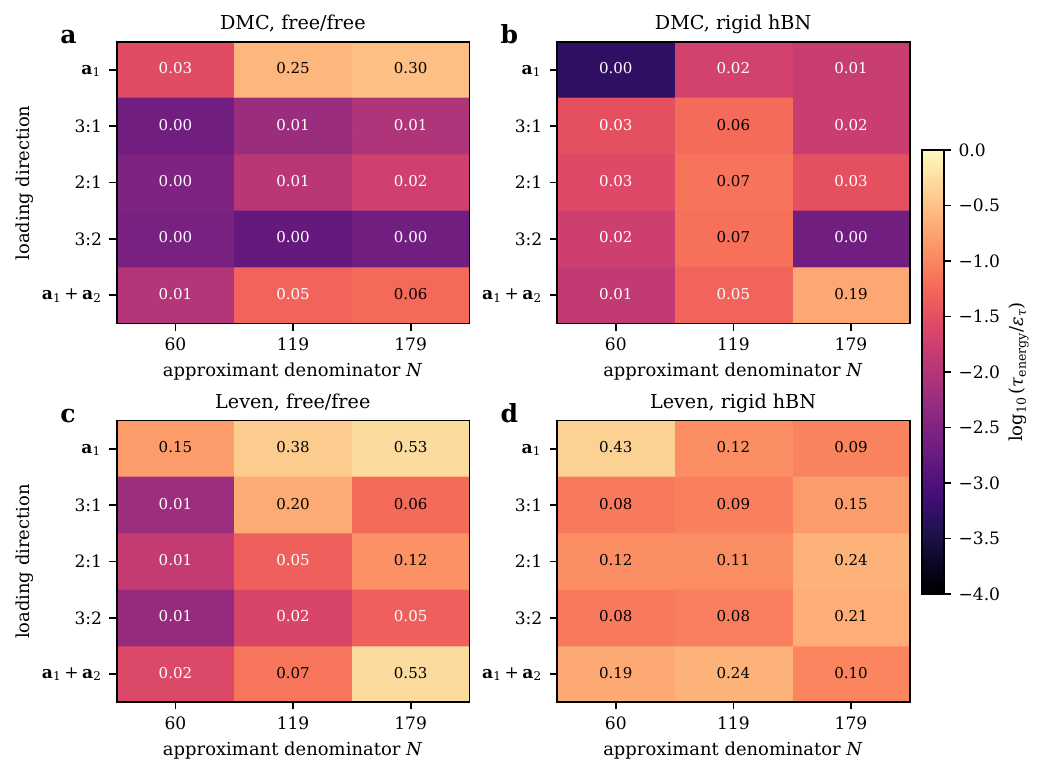}
\caption{
Direction-resolved physical-coupling audit for (a,b) the DMC first-star landscape and (c,d) the 15-harmonic Leven landscape, with free/free and rigid-hBN boundary conditions shown separately. Each entry is $\tau_{\rm energy}/\epsilon_\tau$ for one of five loading directions and three rational approximants. The color scale displays its base-10 logarithm. A resolved barrier requires a ratio greater than one; all 60 paths are below that threshold.
}
\label{fig:s_directional_audit}
\end{figure*}

\section{Strong-coupling finite-size data}

Table~\ref{tab:strong_coupling} collects the complete free/free DMC scan used to test whether a barrier survives increasing approximant size.
\begin{table*}[t]
\caption{Free/free strong-coupling audit along the substrate direction $\bm a_1^{\rm S}$.}
\label{tab:strong_coupling}
\begingroup
\footnotesize
\setlength{\tabcolsep}{4pt}
\begin{ruledtabular}
\begin{tabular}{ccccccc}
$g$ & $p/N$ & $\Lambda$ & max. strain & corrugation (meV/cell) & $\tau_{\rm energy}$ (MPa) & status \\
\hline
20 & $1/60$ & 2.84 & 9.49\% & $7.28\times10^{-14}$ & $1.81\times10^{-9}$ & unresolved \\
20 & $2/119$ & 2.79 & 9.48\% & $5.46\times10^{-14}$ & $1.83\times10^{-9}$ & unresolved \\
40 & $1/60$ & 5.67 & 14.17\% & $6.25\times10^{-10}$ & $1.44\times10^{-6}$ & resolved \\
40 & $2/119$ & 5.58 & 14.15\% & $7.28\times10^{-14}$ & $5.21\times10^{-9}$ & unresolved \\
80 & $1/60$ & 11.35 & 20.70\% & $9.23\times10^{-7}$ & $2.13\times10^{-3}$ & resolved \\
80 & $2/119$ & 11.16 & 20.69\% & $1.94\times10^{-10}$ & $7.43\times10^{-6}$ & unresolved \\
80 & $3/179$ & 11.22 & 20.69\% & $2.93\times10^{-11}$ & $1.81\times10^{-6}$ & unresolved \\
\end{tabular}
\end{ruledtabular}
\endgroup
\end{table*}

The local-strain growth invalidates a quantitative harmonic-elastic interpretation before a size-independent barrier is observed. Consequently these data cannot be fitted to a critical-scaling collapse and do not define $g_c$.

\section{Corner--edge--bulk finite-size extrapolation}

For a fixed flake shape, aspect ratio, loading direction, and preparation protocol, we fit the static depinning force to
\begin{equation}
F_{\rm dep}(A)=a_{\rm c}+b_{\rm e}A^{1/2}+c_{\rm s}A+o(A^{1/2}).
\end{equation}
The corresponding stress is
\begin{equation}
\tau_{\rm dep}(A)=a_{\rm c}A^{-1}+b_{\rm e}A^{-1/2}+c_{\rm s}+o(A^{-1/2}),
\end{equation}
Here $a_{\rm c}$ is a bounded corner force, $b_{\rm e}$ is an edge-envelope coefficient with units of force per length, and $c_{\rm s}$ is a stress. Thus the thermodynamic order parameter is the static area coefficient $c_{\rm s}=\tau_{\rm dep}^{\rm bulk}$, not the finite force. Gao \emph{et al.} report $F_s=b_{\rm e}A^{1/2}$ upper and lower envelopes for polygonal graphene/hBN flakes \cite{Gao2025Edge}. Their published coefficients, with $F_s$ in nN and $A$ in ${\rm nm^2}$, are listed in Table~\ref{tab:gao_edge_coefficients}.
\begin{table}[t]
\caption{Static edge-envelope coefficients $b_{\rm e}$ transcribed from Fig.~4 of Ref.~\cite{Gao2025Edge}; all entries are in $\mathrm{nN/nm}$.}
\label{tab:gao_edge_coefficients}
\begin{ruledtabular}
\begin{tabular}{lcc}
Shape & lower $b_{\rm e}$ & upper $b_{\rm e}$ \\
\hline
Rectangle & 0.65 & 1.34 \\
Square & 0.75 & 1.76 \\
Hexagon & 0.60 & 1.922 \\
Triangle & 1.70 & 2.68 \\
\end{tabular}
\end{ruledtabular}
\end{table}
After division by area, every reported edge envelope decays as $A^{-1/2}$. A nonzero bulk floor $c_{\rm s}$ overtakes it at $A_\times=(b_{\rm e}/c_{\rm s})^2$ in consistent units. The script \texttt{ghbn\_edge\_bulk\_extrapolation.py} records this conversion and the stress flow without refitting plotted data. Gao \emph{et al.} use $a_k+b_kA^{1/2}+c_kA$ for kinetic friction; its $c_k$ is a dissipative surface term and is not interchangeable with the static coefficient $c_{\rm s}$.
The resulting static stress envelopes are shown in Fig.~\ref{fig:s_edge_scaling}.

\begin{figure}[t]
\centering
\includegraphics[width=0.95\linewidth]{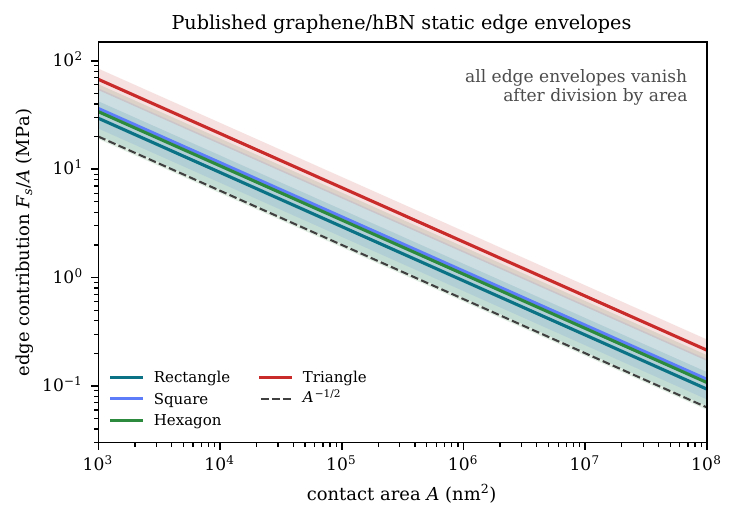}
\caption{
Static edge-envelope coefficients reported by Gao \emph{et al.}, converted from force to stress without refitting their data. Shaded regions span the published lower and upper coefficients for each flake shape. Every envelope follows $A^{-1/2}$ after division by area and therefore vanishes in the thermodynamic stress limit; a nonzero bulk intercept would instead approach a constant.
}
\label{fig:s_edge_scaling}
\end{figure}

\section{Dimensional consistency}

The numerical implementation uses
\begin{equation}
\begin{aligned}
1~{\rm kcal/mol}&=0.0433641153~{\rm eV},\\
1~{\rm N/m}&=0.0624150907~{\rm eV/\Ang^2},\\
1~{\rm eV/\Ang^3}&=1.6021766208\times10^5~{\rm MPa}.
\end{aligned}
\label{eq:unit_conversions}
\end{equation}
The displacement $\bm u$ and collective shift $\bm X$ have units of length, while $\bm G$, $\bm q$, and the sliding-spectrum vector $\bm K$ have units of inverse length. The cell coefficients $E_G$, $\mathcal C_\alpha$, and $\mathcal S_\alpha$ are energies; division by $\Acell$ gives the corresponding GSFE coefficients per area. Both $V_G$ and the two-dimensional elastic moduli have units of energy per area. Since $D(\bm q)=Cq^2$, the elastic kernel has units of energy per length to the fourth power, and
\begin{equation}
|V_G|G_i[D^{-1}(\bm q)]_{ij}G_j
\end{equation}
is dimensionless. The relaxed Fourier coefficient $V^{\rm ren}_{\bm K}$ has units of energy per area, so the spectral diagnostic $\Phi_R=[\sum_{\bm K\ne0}K^2|V^{\rm ren}_{\bm K}|^2]^{1/2}$ has units of energy per volume, equivalent to force per area and hence to shear stress. Likewise, $\tau X$ has units of energy per area in the tilted enthalpy density.

\section{Reproducibility and scope}

The accompanying calculation repository contains the source DOI and Fourier convention, every optimizer report, direct and energy-derived stresses, period-closure errors, displacement and strain diagnostics, and machine-readable DMC--Leven and Gao-scaling summaries. The calculation is zero-temperature and defect-free and uses in-plane harmonic elasticity with either the DMC first star or the 15-harmonic fixed-height Leven spectrum. No claim is made about nonlinear elasticity, dynamically relaxed interlayer height, finite-flake chemistry, polycrystals, pressure, or thermal creep.

The numerical result is a null detection of pinning in the two specified in-plane models, not an experimental zero-friction prediction. All 30 size--direction--boundary paths, six $12\times12$ shift tori, and 50 multi-start endpoints have been evaluated for each adhesion model. Tilted-enthalpy continuation has been completed for all resolved DMC branches found by the constrained searches. A mathematically exhaustive phase assignment would still require a dense angular limit, exclusion of remote branches outside the present search basin, and a fully atomistic out-of-plane calculation.

\bibliographystyle{apsrev4-2}
\bibliography{superlubricity-v16}

\end{document}
